# Supplementary material for: MatchU: Matching Unseen Objects for 6D Pose Estimation from RGB-D Images
Source: arXiv:2403.01517 source file (2024-05-08)
Supplement: Supplementary file 1 [file X_suppl.tex]

\clearpage
\setcounter{page}{1}
\maketitlesupplementary
In this Appendix, we first introduce the detailed network architecture of each module for our method as well as training and inference parameters in Section~\ref{sec:implement}. We then provide the formal definition of the coarse-level loss function in Section~\ref{sec:circle loss}. More visualization results are shown in Section~\ref{sec:vis}. We further conduct an ablation study on the verification and refinement method in Section ~\ref{sec:veri and refine}. Finally, more discussions about the failure cases and limitations are provided in Section ~\ref{sec:limitation}.

\section{Implementation Details} 
\label{sec:implement}
\subsection{Network Architecture}
As shown in Figure ~\ref{fig:supp}, our network consists of two 3D backbones that perform encoding and decoding for the CAD points and depth points respectively, one 2D backbone that embeds textural information from RGB images, and one Latent Fusion Attention Module proposed to fuse the 2D and 3D cues in the coarse-level latent space.
\begin{figure*}[t]
  \centering
  \includegraphics[width=\textwidth]{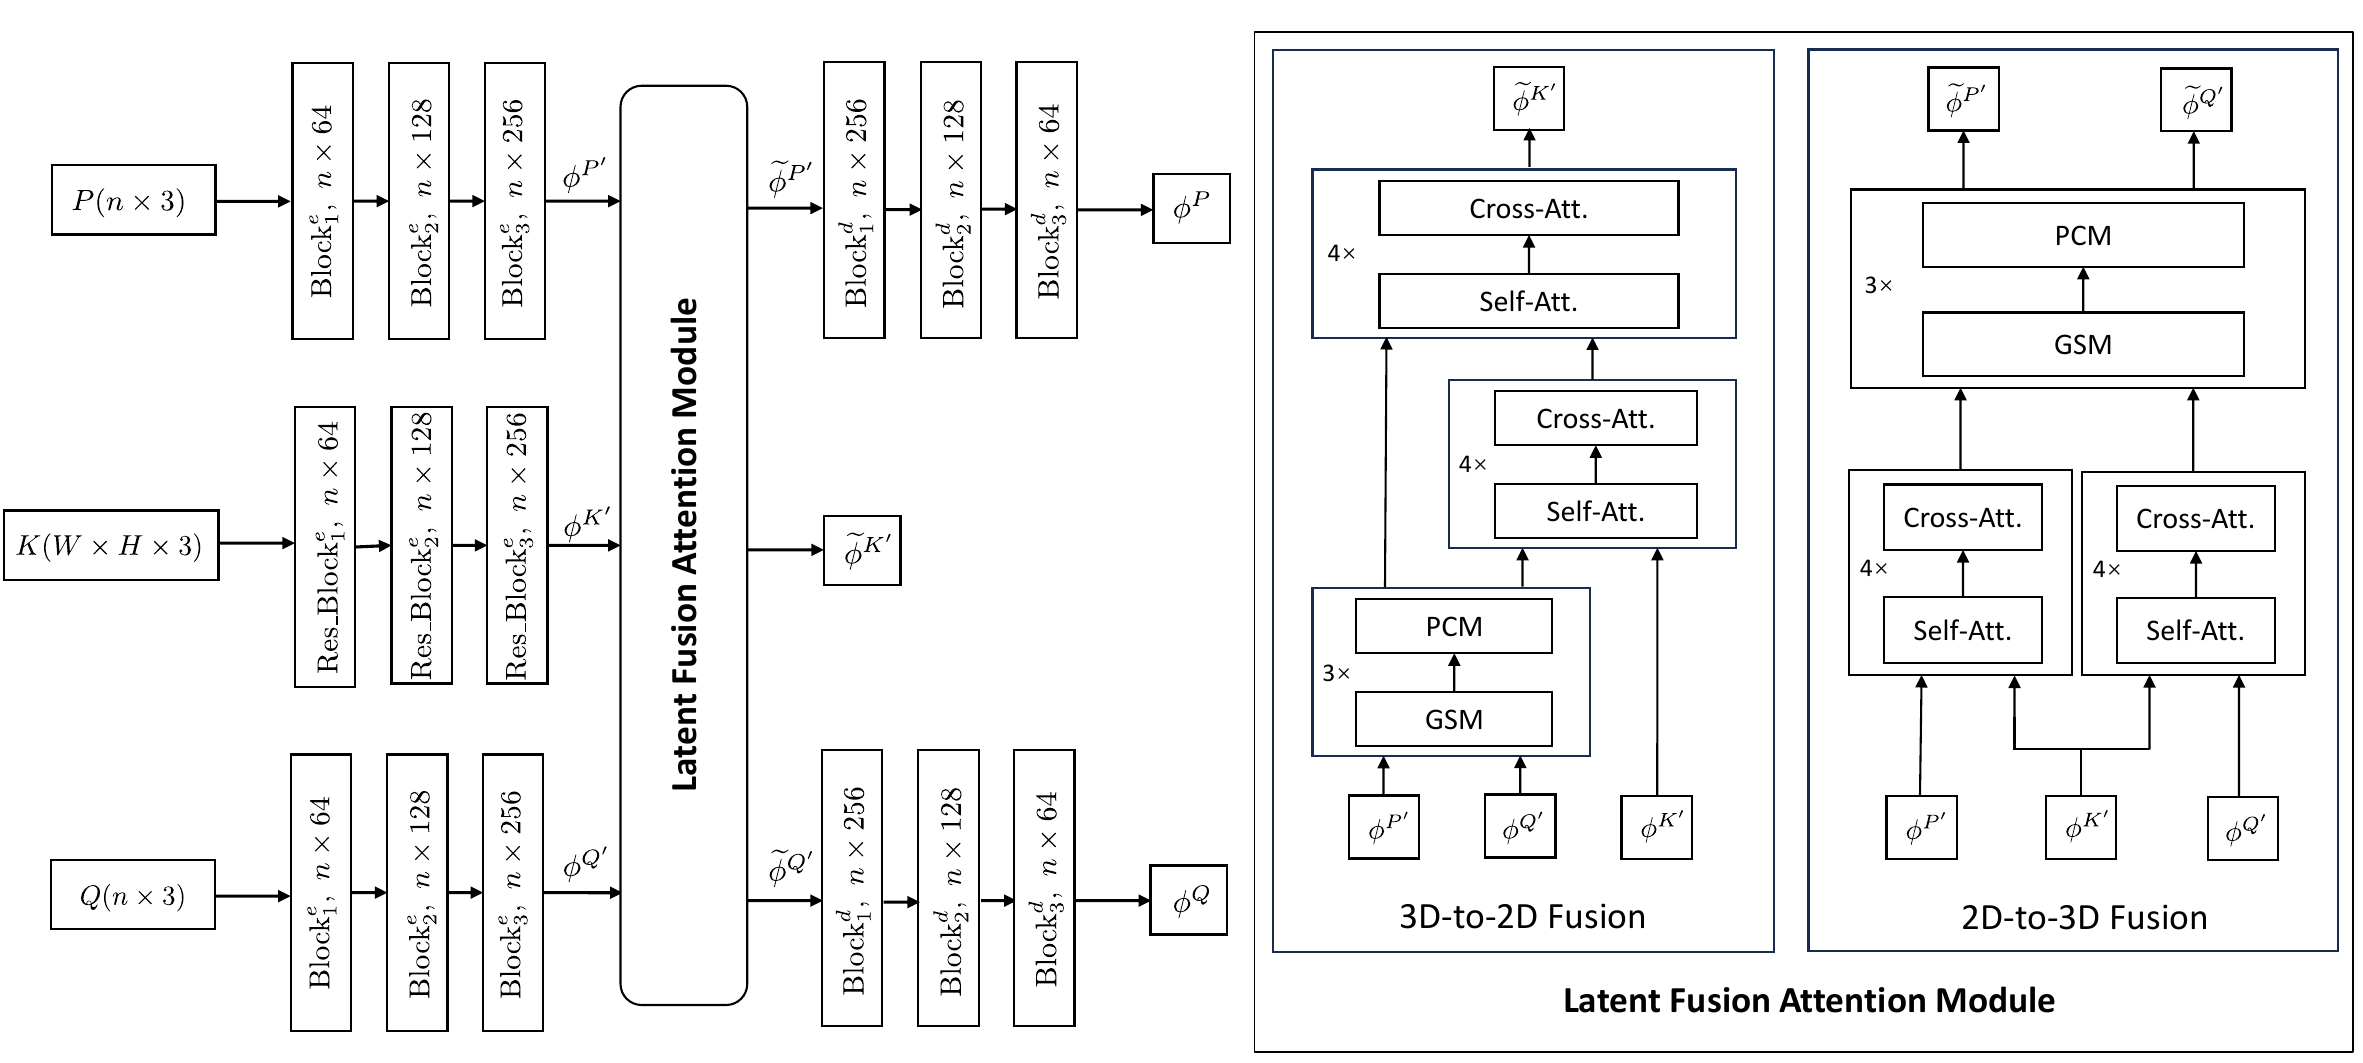}
  \caption{The detailed network architecture of our model.}
  \label{fig:supp}
\end{figure*}

\paragraph{3D Backbone.}
We adjust RoITr~\cite{yu2023roitr} network as our 3D backbone to extract rotation-invariant point descriptors for both the CAD and depth point clouds. For each observed depth image, we sample at most 2048 points as the target point cloud and the same number is applied for sampling points from the CAD model surface as the source point cloud. The 3D encoder-decoder architecture is based on the Point Pair Feature Transformer (PPFTrans). Our point cloud encoder consists of 4 blocks, as shown in Table~\ref{tbl:3dencoder}, each block consists of an Attentional Abstraction Layer (AAL) for downsampling and abstraction and a PPF Attention Layers (PALs) for local geometry encoding and context aggregation. Both layers are in the same design with RoITr. We use the stride of 1,4, 2, and 2 for the encoder blocks respectively. The encoder blocks finally down-sample the point clouds into 128 superpoints with 256 feature dimensions. The decoder is also built by 4 blocks, as shown in Table~\ref{tbl:3ddecoder}, each block is made of a
Transition Up Layer (TUL) that performs upsampling and context aggregation, as well as a PAL which enhances the highly-representative learned context.

\begin{table}[ht!]
\centering
\resizebox{\columnwidth}{!}{
\begin{tabular}{c|c|c}
\toprule
Stage &Block &Operation  \\
\midrule
\midrule
Input & &${P}\in \mathbb{R}^{n\times1}$  \\
\cline{1-3}
\multirow{8}{*}{Encoder} &\multirow{2}{*}{$\text{Block}^e_{1}({P})\rightarrow{P}_1$} &AAL$(n \times 1) \rightarrow n\times 64$\\

& &PAL$(n \times 64) \rightarrow n\times 64$\\
\cline{2-3}

&\multirow{2}{*}{$\text{Block}^e_{2}({P}_1)\rightarrow{P}_2$} &AAL$(n \times 64) \rightarrow n / 4\times 128$ \\

& &PAL$(n / 4 \times 128)\rightarrow n / 4\times 128$\\
\cline{2-3}

&\multirow{2}{*}{$\text{Block}^e_{3}({P}_2)\rightarrow{P}_3$} &AAL$(n / 4 \times 128) \rightarrow n / 8\times 256$  \\

& &PAL$(n / 8 \times 256) \rightarrow n / 8\times 256$ \\
\cline{2-3}

&\multirow{2}{*}{$\text{Block}^e_{4}({P}_3)\rightarrow{P}'$} &AAL$(n / 8 \times 256) \rightarrow n / 16\times 256$ \\

& &PAL$(n / 16 \times 256) \rightarrow n / 16\times 256$\\
\midrule

Output & &$P'~~,~~\mathcal{\phi}^{p'}$  \\
\bottomrule

\end{tabular}
}
\caption{Detailed architecture of our 3D encoder.}
\label{tbl:3dencoder}
\end{table}

\begin{table}[ht!]
\centering
\resizebox{\columnwidth}{!}{
\begin{tabular}{c|c|c}
\toprule
Stage &Block &Operation  \\
\midrule
\midrule
Input & &${P'}\in \mathbb{R}^{n/16\times256}$  \\

\midrule
\multirow{8}{*}{Decoder} &\multirow{2}{*}{$\text{Block}^d_{4}({P}^\prime)\rightarrow\hat{{P}}_4$} &TUL $(n/16 \times 256) \rightarrow n/16\times 256$\\

& &PAL: $n/16\times 256 \rightarrow n/16\times 256$\\
\cline{2-3}

&\multirow{2}{*}{$\text{Block}^d_{3}(\hat{{P}}_4, {P}_3)\rightarrow\hat{\mathcal{P}}_3$} &TUL$(n/16 \times 256,\; n/8 \times 256)\rightarrow n / 8\times 256$  \\

& &PAL$(n / 8 \times 256)\rightarrow n / 8\times 256$ \\
\cline{2-3}

&\multirow{2}{*}{$\text{Block}^d_{2}(\hat{{P}}_3, {P}_2)\rightarrow\hat{\mathcal{P}}_2$} &TUL$(n / 8 \times 256,\;n / 4\times 128)\rightarrow n / 4\times 128$  \\

& &PAL$(n / 4 \times 128) \rightarrow n / 4\times 128$ \\
\cline{2-3}

&\multirow{2}{*}{$\text{Block}^d_{1}(\hat{\mathcal{P}}_2, {P}_1)\rightarrow\hat{{P}}$} &TUL$(n / 4 \times 128,\; n\times 64)\rightarrow n\times 64$ \\

& &PAL$(n \times 64)\rightarrow n \times 64$\\
\midrule
Output & &$\hat{P}~~,~~\mathcal{\phi}^{p}$  \\
\bottomrule

\end{tabular}
}
\caption{Detailed architecture of our 3D decoder.}
\label{tbl:3ddecoder}
\end{table}

\paragraph{2D Backbone.}
For learning the textural information from the RGB images, we follow the implementation of LoFTR~\cite{sun2021loftr} and use a modified ResNet18~\cite{he2016deep} as the 2D backbone network. It consists of 3 convolutional blocks which down-sample the input image into $\frac{W}{2} \times \frac{H}{2}$, $\frac{W}{4} \times \frac{H}{4}$, $\frac{W}{8} \times \frac{H}{8}$ feature maps respectively.  The feature map with resolution of $\frac{W}{8} \times \frac{H}{8} \times 256$ is then flattened and encoded with the positional embeddings. Same as LoFTR, the 2D extension of the absolute sinusoidal positional encoding is adopted. Finally, the superpixels from 2D branch are further fused with the obtained 3D superpoint features by the proposed Latent Fusion Attention Module. 

\paragraph{Global Transformer.}
We aggregate the global context with a Global Transformer proposed in ~\cite{roitr}. It consists of 3 blocks, each block is a sequence of a geometry-aware self-attention module~(GSM) and a position-aware cross-attention module~(PCM). The global transformer encodes the spatial cues from both CAD and depth point clouds and enhances the geometric features for both sides.

\paragraph{Latent Fusion Attention Module.}
As introduced in the main text, our Latent Fusion Attention Module consists of two types of transformers, \ie Fusion Transformer and Global Transformer. The detailed network structure of this module is shown in the right part of Figure~\ref{fig:supp}. For the global transformers, we follow the design of ~\cite{roitr}. It consists of 3 blocks, each block is a sequence of a geometry-aware self-attention module~(GSM) and a position-aware cross-attention module~(PCM). The global transformer encodes the spatial cues from both CAD and depth point clouds and enhances the geometric features for both sides.
For the fusion transformers, We follow~\cite{sun2021loftr} to design the attention layers and use 4 self- and cross-attention layers in each transformer block. In the Latent Fusion Attention Module, we obtain the features of 2D and 3D in different fusion branches. For 3D-to-2D fusion branch, we first use a global transformer to aggregate the cross-frame context between CAD and depth superpoints, then we fuse the obtained global-aware depth and CAD superpoint features with the 2D local features respectively, from which we obtain the fused 2D superpixel features $\widetilde{\phi}^{K'}$. For 2D-to-3D fusion branch, we first encode 2D features into CAD and depth superpoint features respectively, then we aggregate the fused CAD and depth features with a global transformer and obtain the global-aware 3D superpoint features $\widetilde{\phi}^{P'}$ and $\widetilde{\phi}^{Q'}$.

\subsection{Training and Inference Parameters}
During training, all the objects are normalized into a sphere with a radius of 0.1m, and we let $\lambda_{r}$ to be 0.01 and 0.005 for coarse and fine matching respectively. We set $\lambda_b$ as 0.3 and $\gamma_c$ as 0.5 by default, and adopt an Adam~\cite{kingma2014adam} optimizer with an initial learning rate of 1e-4, which is exponentially decayed by 0.05 after each epoch. We train our model around 1M iterations with a batch size of 2 on two RTX4090 GPUs, while the model is tested without CPU parallel and with a batch size of 1. During inference, we set $\kappa=128$, $s=64$ and $\eta=20$ by default. For the testing under the condition of unseen object localization, we adopt a CAD-based novel object segmentation method~\cite{nguyen2023cnos} to localize the objects in our input RGB-D images. 
For the evaluation of 6D pose with instance-level localization, we take the existing detection results from the methods~\cite{zeropose,Li_2019_ICCV,Sundermeyer_2020_CVPR}. To boost the performance, we scale up $\eta=64$ to achieve more accurate results in comparison to some baselines\cite{gcpose,megapose}.
In all the experiments, we select 128 superpoint correspondences with the highest confidence scores as the coarse-level superpoint matching.

\section{Loss Function}
\label{sec:circle loss}
We explain the detailed Circle Loss~\cite{circle} for the coarse-level matching between the superpoints and superpixels. The Circle Loss re-weight each similarity score
under supervision, and is compatible with both class-level labels and pair-wise labels.  Following ~\cite{Qin_2022_CVPR}, we use the overlaps between the corresponding superpoints as the similarity re-weighting score. For each superpoint $p'_{i}\in P'$, and $q'_{j}\in Q'$, we can calculate the overlap $\mathcal{V}$ between $p'_{i}$ and $q'_{j}$ as:
\begin{equation}
  \label{eq:overlap}
    \mathcal{V}(p'_{i}, q'_{j}) = \frac{|\{\hat{p'}_{u}\in\hat{P'}_{i} \mid \exists\ \hat{q'}_{v}\in \hat{Q'}_{j} 
    : \hat{p'}_{u} \leftrightarrow \hat{q'}_{v}\}|}{|\{\hat{p'}_{u} \in \hat{P'}_{i}\}|},
\end{equation}

\noindent where $\leftrightarrow$ denotes the correspondence relationship. $\hat{P'}_{i}$ is 
the group of points from $P'$ assigned to $p'_{i}$ by Point-to-Node grouping strategy~\cite{yu2021cofinet}, and $\hat{Q'}_{j}$ means the same for $Q^\prime$.

A pair of superpoints $p'_{i}$ and $q'_{j}$ are considered as a positive pair if and only if $\mathcal{V}(p'_{i}, q'_{j}) > \tau_r$, where $\tau_r$ is the threshold of the overlap.
We sample a positive set of superpoints from $Q'$, denoted as 
$\mathcal{E}^P_i = \{{q}^\prime_j \in {Q}^\prime \mid \mathcal{V}({p}^\prime_i, 
{q}^\prime_j) > \tau_r\}$, 
and a negative set of superpoints 
$\mathcal{F}^P_i = \{{q}^\prime_j \in {Q}^\prime \mid \mathcal{V}({p}^\prime_i, {q}^\prime_j) =0\}$. 
Then for ${P}^\prime$, the coarse-level superpoint matching loss is computed as: 
\begin{align}
    &\mathcal{L}^{P'}_{c} = \frac{1}{n^\prime}\sum_{i=1}^{n^\prime}\text{log}[1 + \\
    &\sum_{{q}^\prime_j \in \mathcal{E}^P_i} {\exp({v^j_i\beta^{i, j}_e(d^j_i-\Delta_e)}} ) 
    \sum_{{q}^\prime_k\in \mathcal{F}^P_i}{\exp(\beta^{i, k}_f(\Delta_f-d^k_i))}],\nonumber
\label{eq:coarse}
\end{align}
\noindent with $v^j_i = \mathcal{V}({p}^\prime_i, 
{q}^\prime_j)$ and $d^j_i = \lVert\widetilde{{\phi_{p'_{i}}}} - \widetilde{{\phi_{q'_{j}}}} \rVert_2$. 
$\Delta_e$ and $\Delta_f$ are the positive and negative margins.
$\beta^{i, j}_e = \gamma(d^j_i - \Delta_e)$ and $\beta^{i, k}_f=\gamma(\Delta_f - d^k_i)$ are the weights individually
determined for different samples, with $\gamma$ as a hyper-parameter. 
This Circle Loss minimizes the corresponding latent features and maximizes the incorresponding features among the superpoints and superpixels, establishing the cross-modality matches on coarse-level latent space.

\section{Verification and Refinement}
\label{sec:veri and refine}
As introduced in the main text, our model is able to produce multiple pose hypotheses from the correspondences. We consider the availability of 2D RGB images and 3D point clouds information and employ both of them to perform verification for our pose hypotheses. As for 3D, we calculate the one-directional chamfer distance between the transformed CAD model and the lifted depth map as the score of 6D pose estimation. Specifically, we first transform the CAD point cloud with our predicted pose hypotheses respectively. For each point in the CAD points, we find the nearest point in the depth points and then measure the Euclidean distance between the CAD point and its nearest reference point. Finally, the pose hypothesis with the smallest mean distance over the CAD points is considered to be the final prediction. However, this measurement is not accurate because a low 3D point-distance-based score does not guarantee an accurate pose. As a complementary option, we also consider using 2D information as verification. We adopt a pre-trained scoring network the same as ~\cite{megapose}. It takes a pair of RGB image crop and its coarse 6D pose prediction as input and estimates a confidence score for each input pair. Training with a large amount of image-pose pairs, this simple deep network is able to reject the outlier pose predictions. In addition to the 2D and 3D verification, we further boost the performance with a standard ICP procedure.
In Table \ref{tbl:ablation refine}, we evaluate the effect of RGB verification and ICP refinement for our method on LM-O dataset. 
We observe that the RGB verification can help reject the outlier hypotheses, and ICP can refine our estimated poses even further. 
By adopting both the RGB verification and ICP refinement, our method achieves the best performance.

\begin{table}[th]
\centering
% \vspace{-0.5cm}
\begin{tabular}{cccc}
   \toprule[1.1pt]
{RGB Verification} & {ICP} & {AR} \\ \hline
& & 56.2  \\
\ding{51} &  & 61.1 \\ 
& \ding{51} & 63.5  \\ 
\ding{51} & \ding{51} & 64.4 \\ 
\bottomrule[1.1pt]
\end{tabular}
\caption{\textbf{Ablation study on verification and refinement of our method on LM-O dataset.}}

\label{tbl:ablation refine}
\end{table}

\section{More Qualitative Results}
\label{sec:vis}
We show more qualitative results on TUD-L, IC-BIN and YCB-V datasets in Figure~\ref{fig:supp_tudl}, ~\ref{fig:supp_icbin}, and  ~\ref{fig:supp_ycbv} respectively.

\section{Limitations}
\label{sec:limitation}
\paragraph{Failure Cases.}
We show some of our failure cases in Figure~\ref{fig:supp_failure}. Our method fails to predict the objects in the first two columns because of different levels of external occlusion, which are reasonable since the observed part is limited by the viewpoint in both texture and depth. In the third column, the orientation of the banana is wrong although the predicted partial pose is well-aligned. This is because the distinctive part is unseen and causes ambiguity when matching the partial observation. We expect this ambiguity can be solved by increasing the resolution of our descriptors. Another failure case is shown in the fourth column, our method predicts the pose of the milk box upside down without external occlusion, which happens because of the highly symmetric texture and geometry presented in the observed part, introducing ambiguity when matching the descriptors with high similarity.

\paragraph{Further Discussions.}
Our method produces generic descriptors by fusing the 2D textural and 3D geometric information in the latent space. It captures the symmetry distribution automatically without external annotation. However, our method still needs further improvement in the verification of the correspondences and poses, especially when matching those highly symmetric objects that present similar features. Feasible solutions could be introducing a spatial consistency mechanism to filter out ambiguous correspondences or some learning-based and graph search methods. By puring the correspondences, higher quality of the pose hypotheses can be produced. On the other hand, instance mask prediction can also be involved in our pipeline by adding an additional output channel in our 2D branch, while multi-task training may also cause potential risks for representation learning. Finally, directly matching the objects to a raw scene without detection or segmentation is also a challenging and interesting direction for future research.

\begin{figure*}[t]
  \centering
  \includegraphics[width=\textwidth]{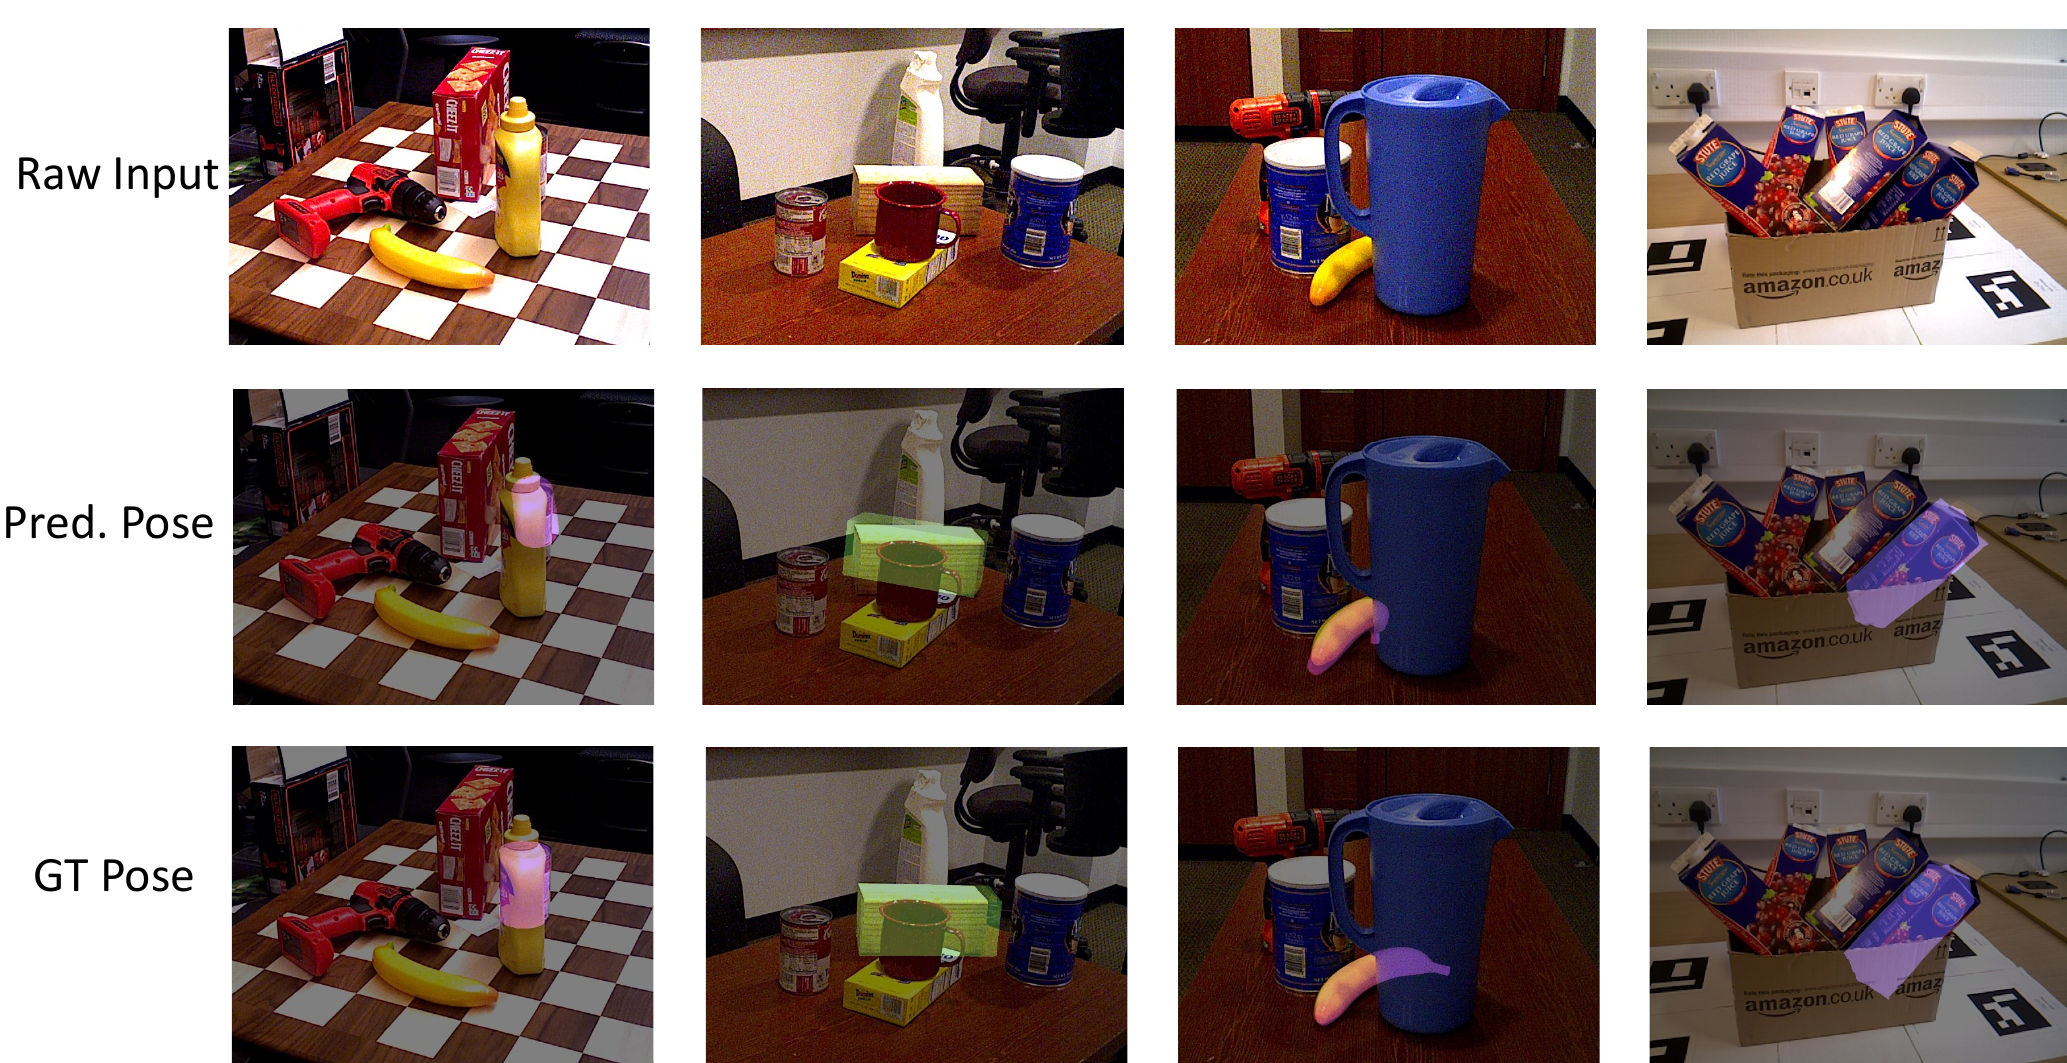}
  \caption{Failure case visualization of our method.}
  \label{fig:supp_failure}
  \vspace{2cm}
\end{figure*}

\begin{figure*}[t]
  \centering
  \includegraphics[width=\textwidth]{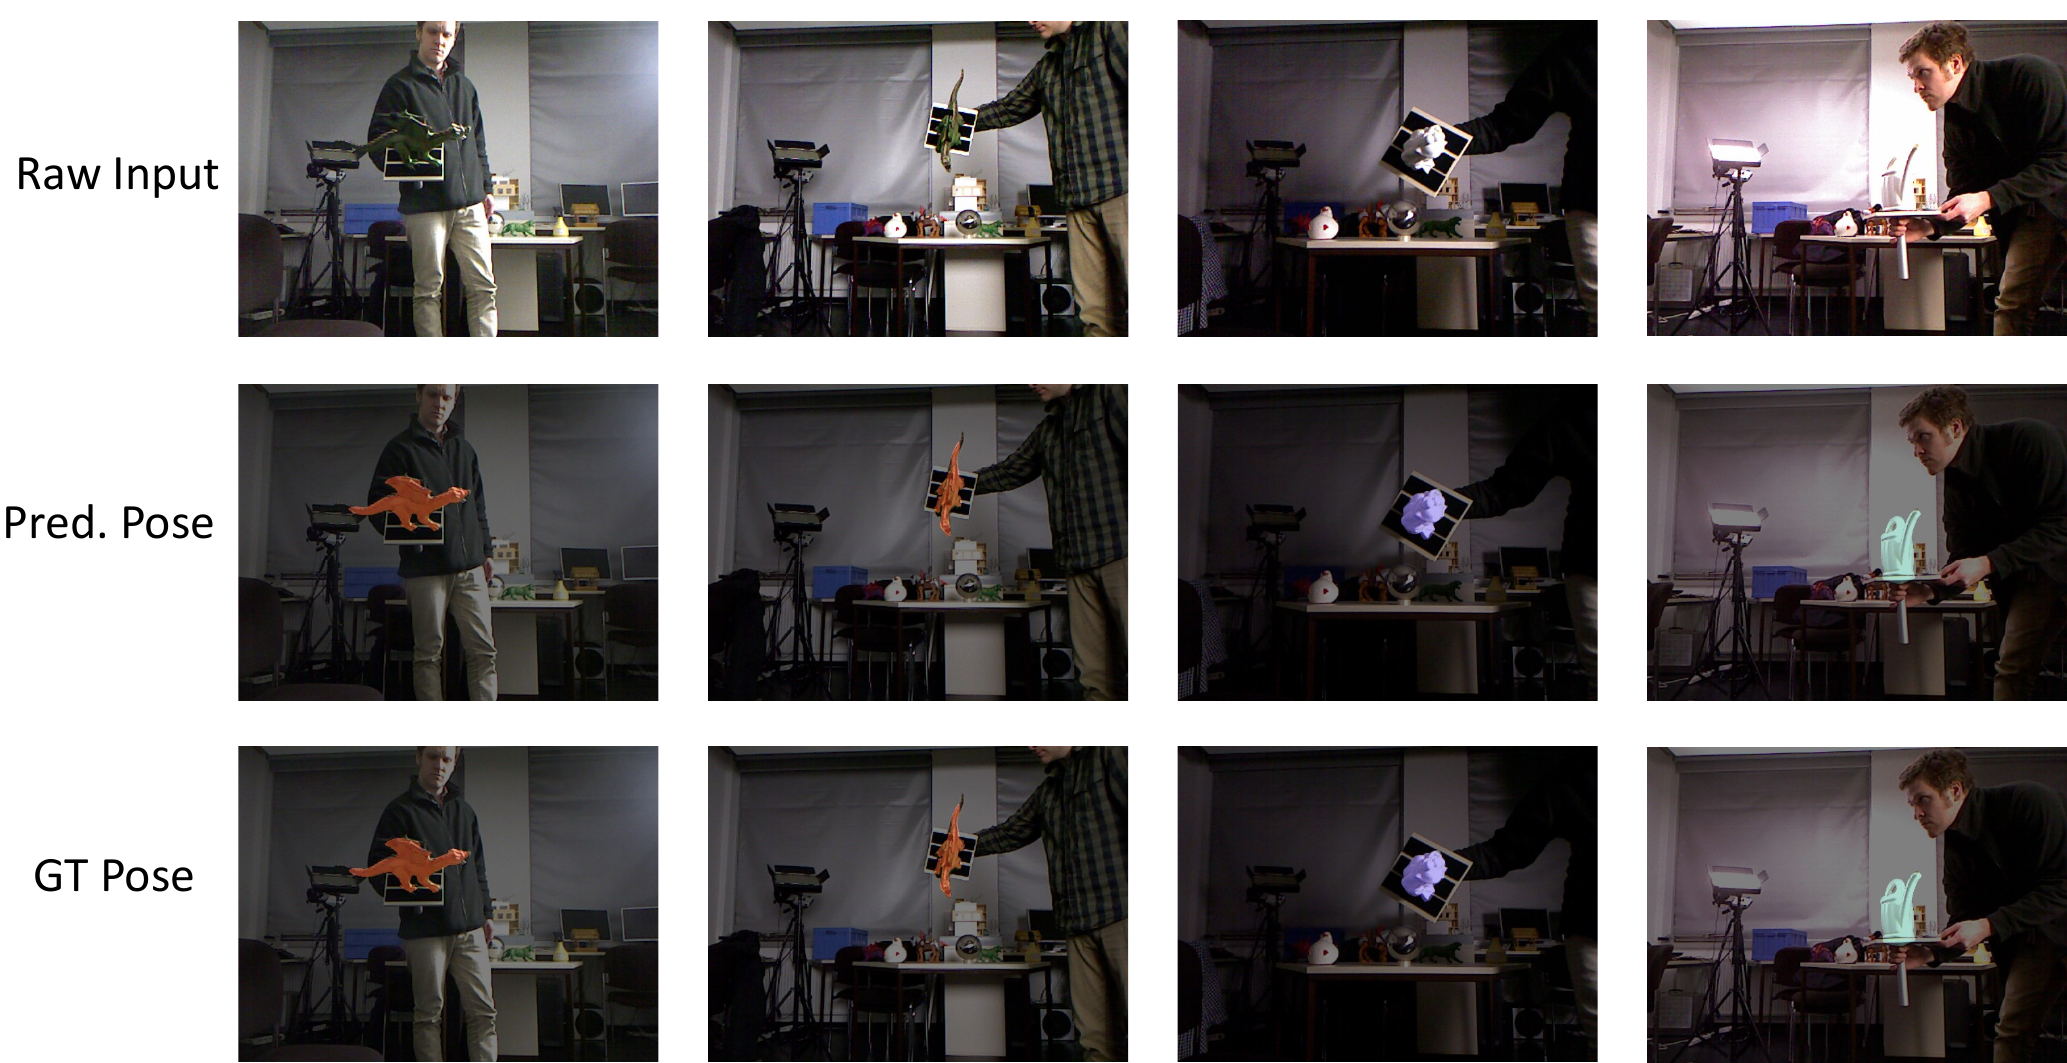}
  \caption{Visualization results of our method on TUD-L dataset.}
  % \vspace{5cm}
  \label{fig:supp_tudl}
  
\end{figure*}
\begin{figure*}[t]
  \centering
  \includegraphics[width=\textwidth]{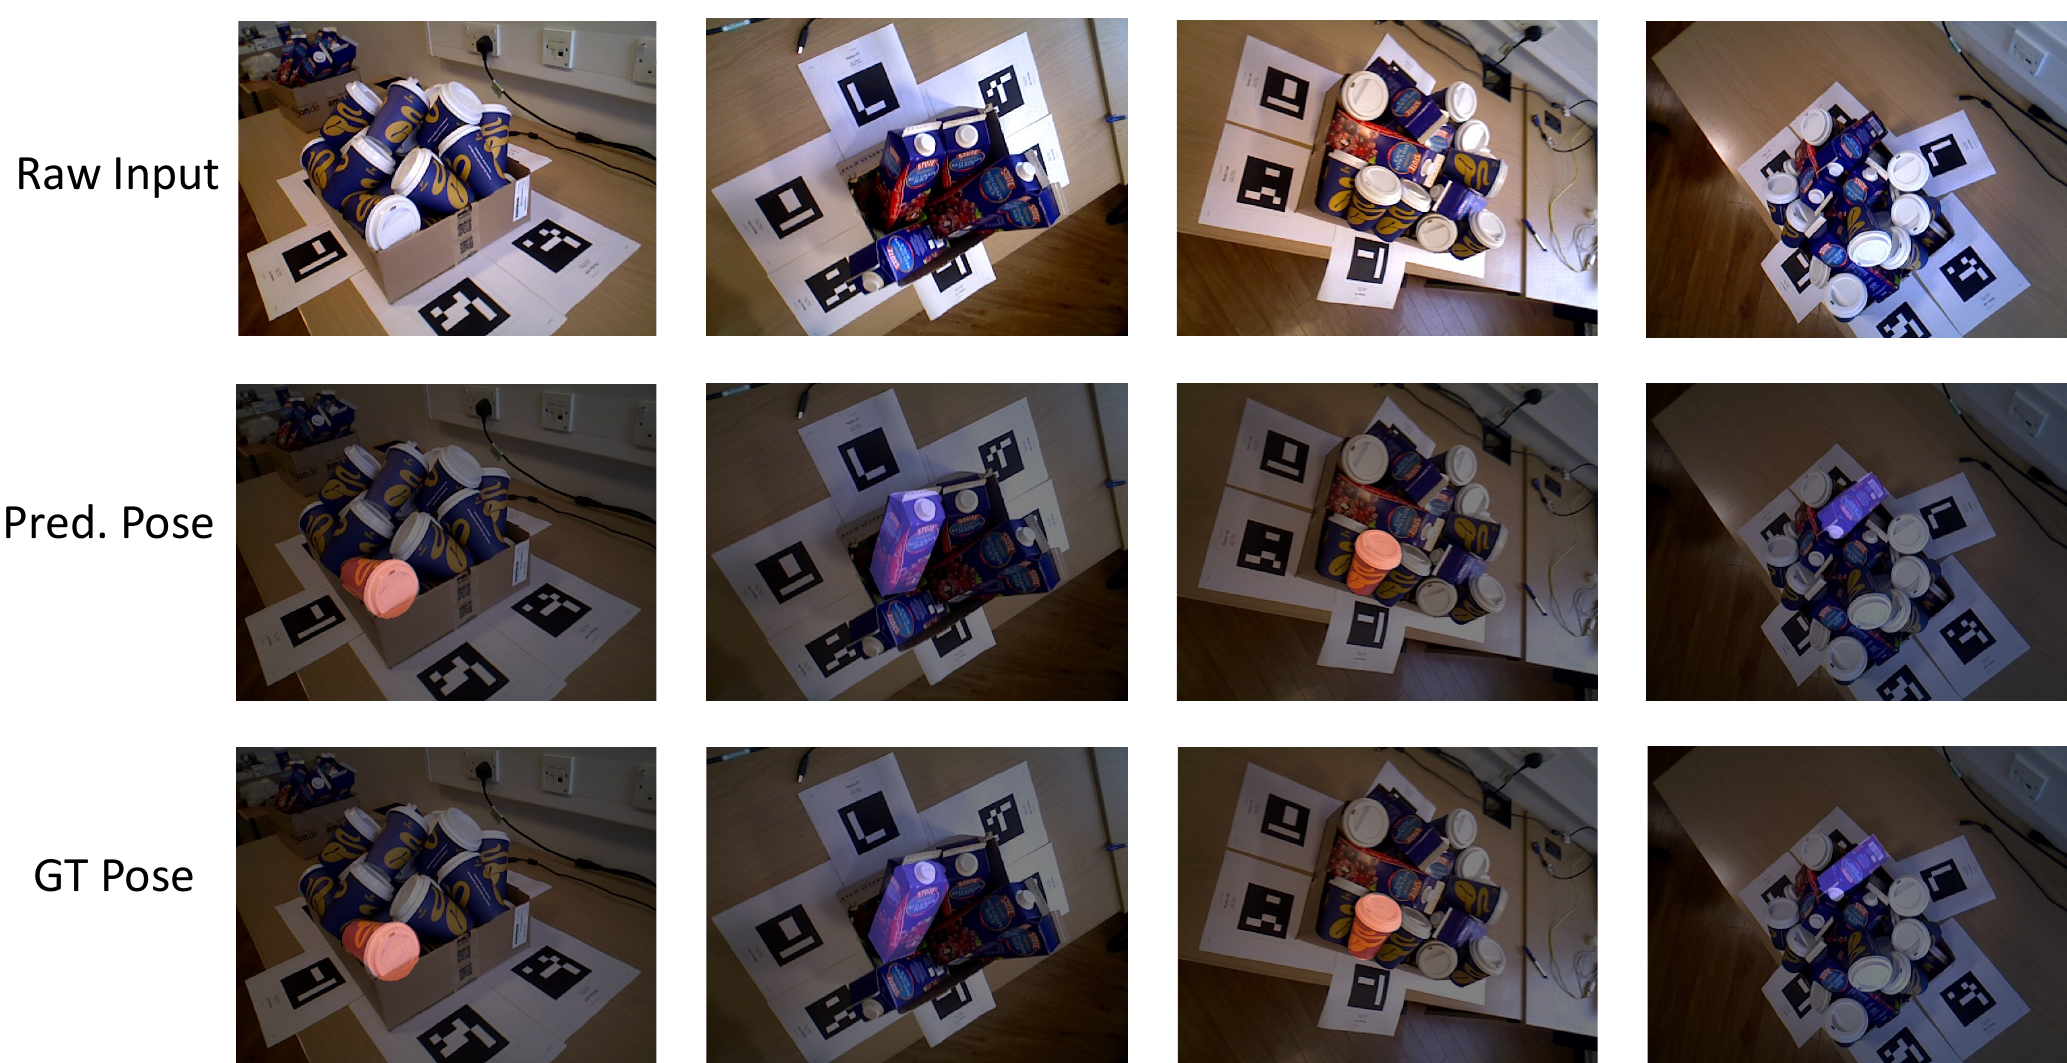}
  \caption{Visualization results of our method on IC-BIN dataset.}
  \label{fig:supp_icbin}
\end{figure*}

\begin{figure*}[t]
  \centering
  \includegraphics[width=\textwidth]{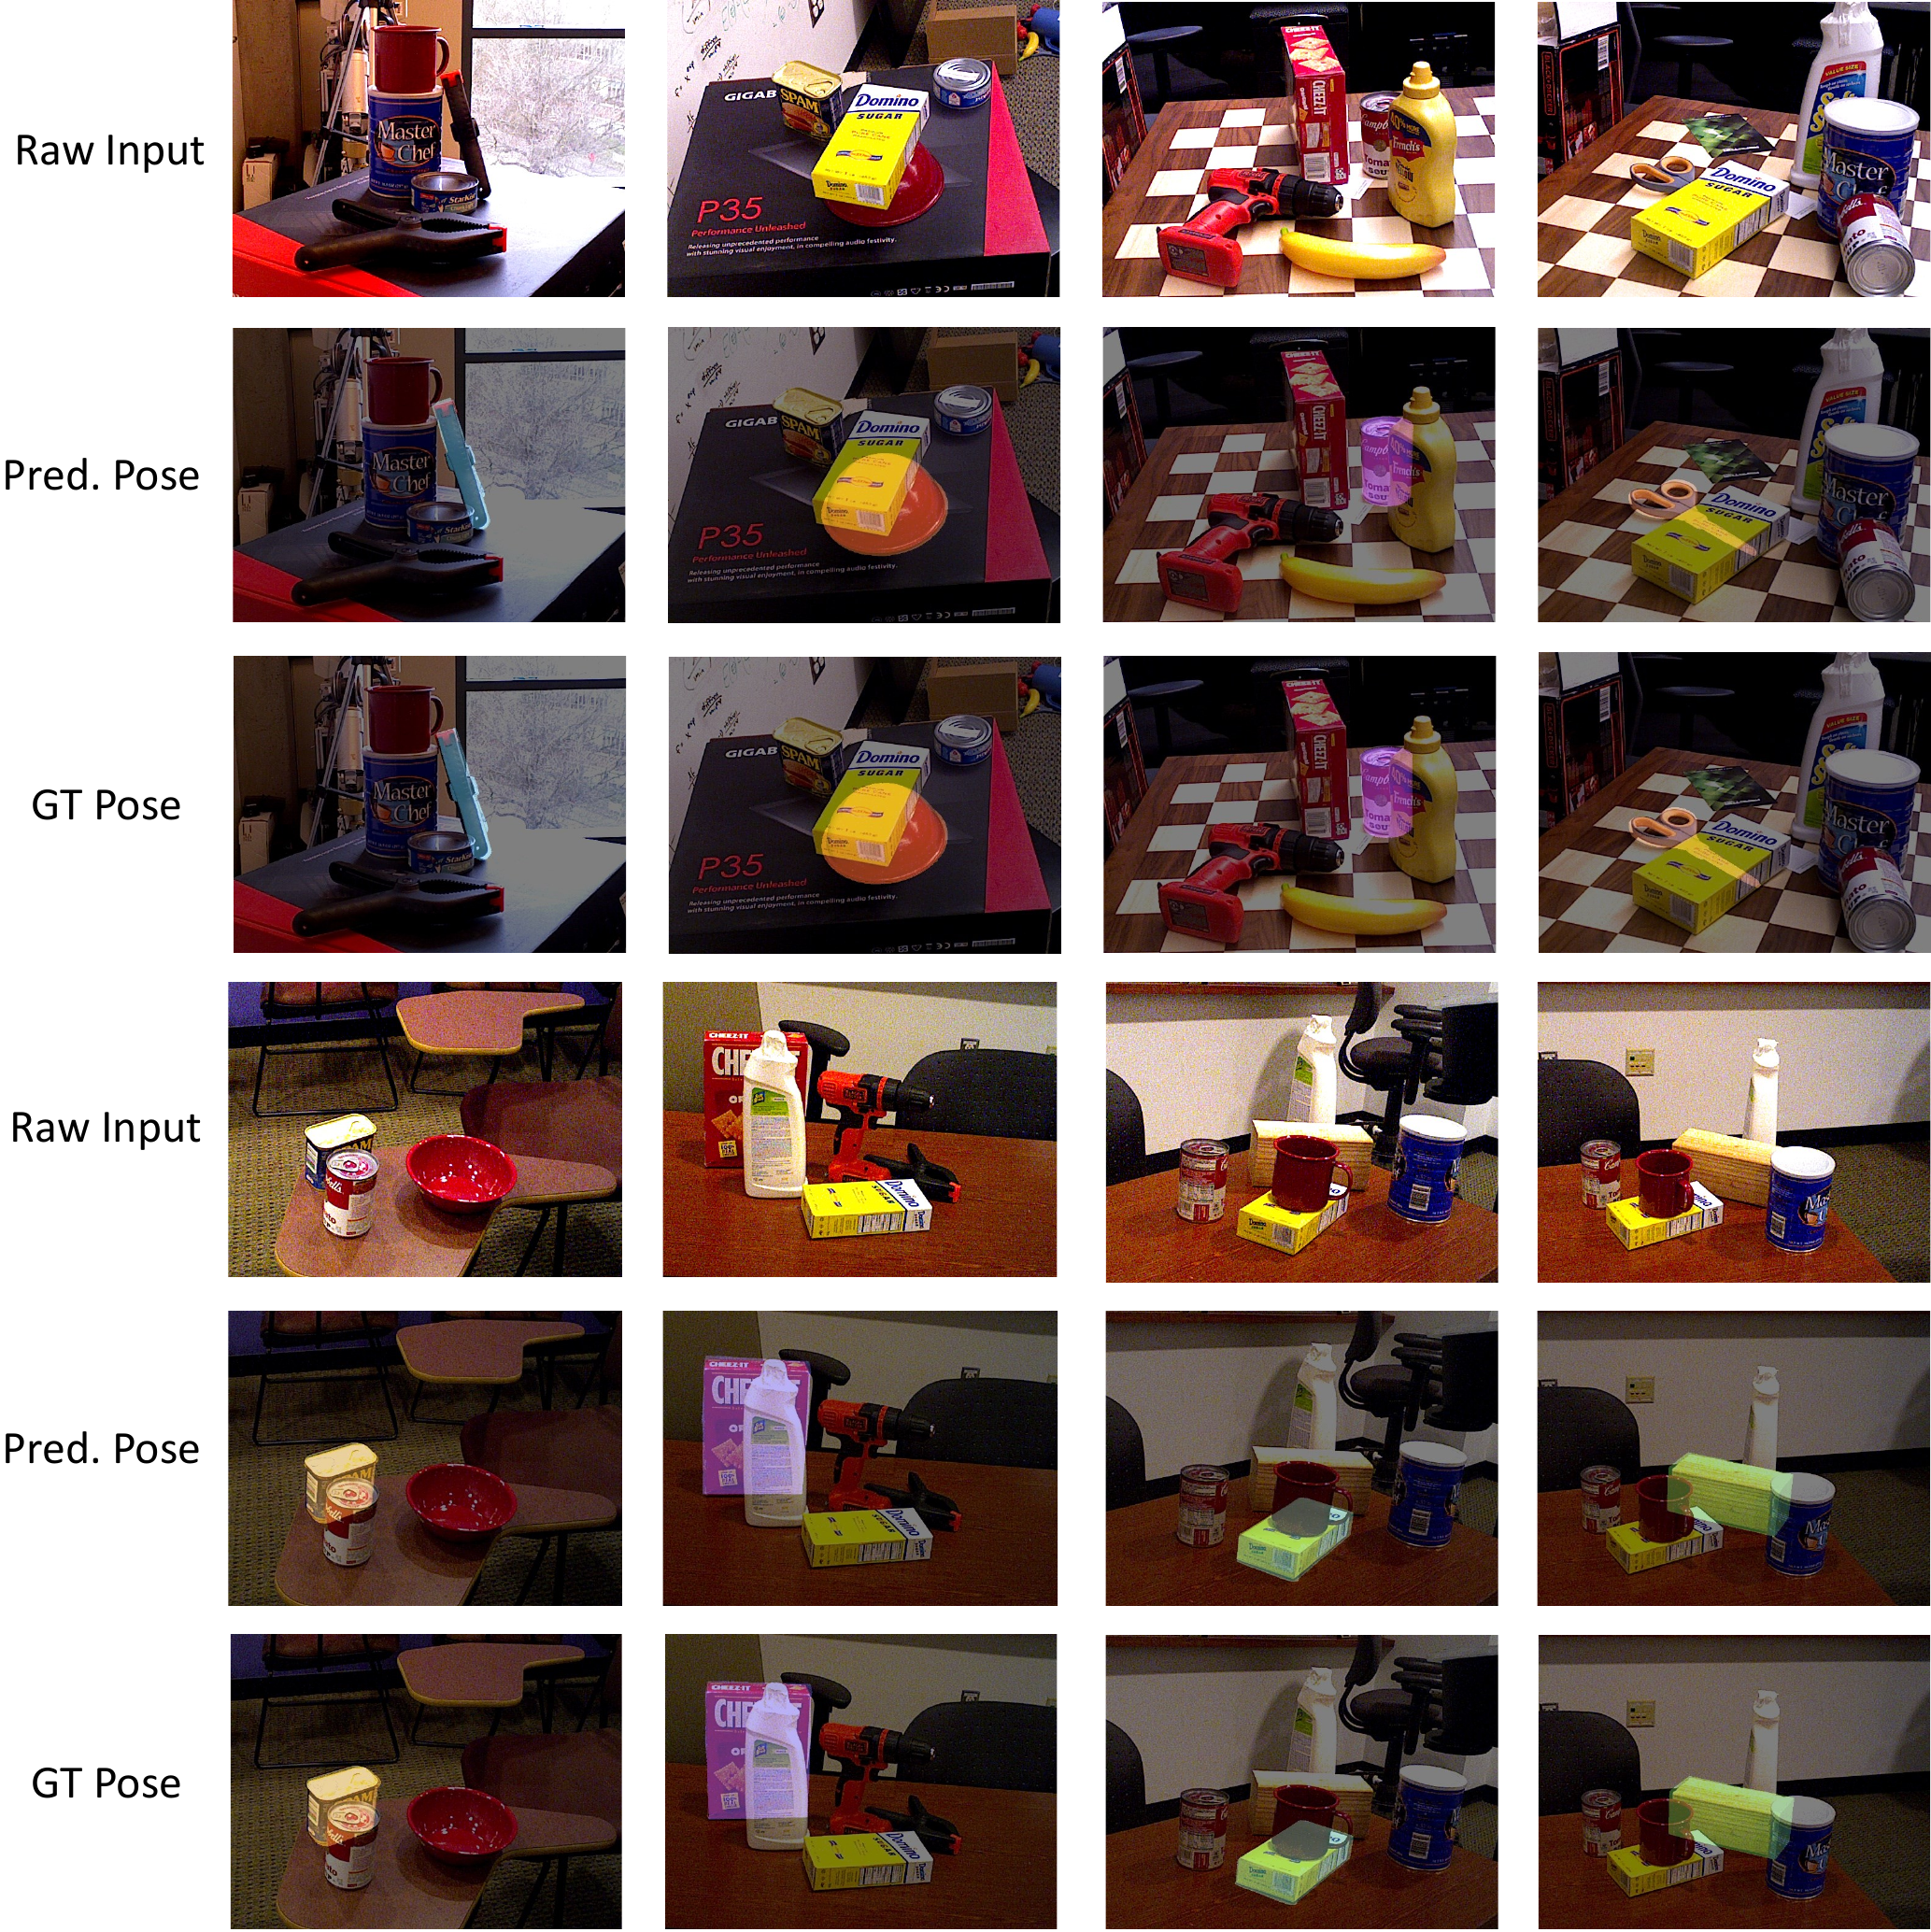}
  \caption{Visualization results of our method on YCB-V dataset.}
  \label{fig:supp_ycbv}
\end{figure*}

Object 6 DoF pose estimation is a crucial aspect in the realms of computer vision and robotics, which has witnessed considerable attention, particularly with the advent of deep learning methodologies. Recent years have seen the emergence of diverse techniques, encompassing 2D-3D or 3D-3D descriptor-matching approaches, template-based methods, direct-regression methods, etc. However, challenges persist in scenarios involving textureless objects, occlusion, and cluttered backgrounds. This thesis introduces a novel pose estimation method based on diffusion models, which have demonstrated notable success in image synthesis tasks. The objective is to leverage the strengths of diffusion models,
such as their scalability to large-scale data and the diversity of generation, to address the complexities inherent in 6 DoF pose estimation. A comprehensive diffusion framework is proposed, utilizing a single RGB-D image to generate multiple hypotheses for the 6 DoF pose of an object. The proposed method is rigorously evaluated on real-world datasets featuring noise and occlusion. Results indicate that our approach achieves comparable performance with state-of-the-art methods, highlighting its effectiveness in challenging scenarios. This study not only contributes a novel perspective to pose estimation but also underscores the potential of diffusion models in advancing the state of the art in this critical domain.

% 
% To split the supplementary pages from the main paper, you can use \href{https://support.apple.com/en-ca/guide/preview/prvw11793/mac#:~:text=Delete%20a%20page%20from%20a,or%20choose%20Edit%20%3E%20Delete).}{Preview (on macOS)}, \href{https://www.adobe.com/acrobat/how-to/delete-pages-from-pdf.html#:~:text=Choose%20%E2%80%9CTools%E2%80%9D%20%3E%20%E2%80%9COrganize,or%20pages%20from%20the%20file.}{Adobe Acrobat} (on all OSs), as well as \href{https://superuser.com/questions/517986/is-it-possible-to-delete-some-pages-of-a-pdf-document}{command line tools}.
